# Supplementary material for: Explainable Anomaly Detection in 5G Networks through Continuous Time Graphs
Source: arXiv:2611.06225 source file (2026-11-04)
Supplement: Supplementary file 1 [file appendix.tex]

\begin{table*}[t]
\centering
\small
\renewcommand{\arraystretch}{1.2}
\begin{tabular}{|l|c|c|c|c|c|c|c|c|c|c|}
\hline
\textbf{Feature} &
\rotatebox{90}{\textbf{Applicative MITM}} &
\rotatebox{90}{\textbf{Applicative Scan}} &
\rotatebox{90}{\textbf{API Fuzzing}} &
\rotatebox{90}{\textbf{Session Establishment Flood}} &
\rotatebox{90}{\textbf{Session Deletion Flood}} &
\rotatebox{90}{\textbf{SEID Fuzzing}} &
\rotatebox{90}{\textbf{Session Modify Drop}} &
\rotatebox{90}{\textbf{Session Modify Duplicate}} &
\rotatebox{90}{\textbf{Uplink Spoofing}} &
\rotatebox{90}{\textbf{PFCP in GTP}} \\
\hline
ip\_dst & \ding{54} & \ding{54} & \ding{54} & \ding{54} & \ding{54} & \ding{54} & \ding{54} & \ding{54} & \ding{54} & \ding{54} \\ \hline
ip\_src & \ding{54} & \ding{54} & \ding{54} & \ding{54} & \ding{54} & \ding{54} & \ding{54} & \ding{54} & \ding{54} & \ding{54} \\ \hline
gtp.ip\_dst & & & & & & & & & \ding{54} & \\ \hline
gtp.ip\_src & & & & & & & & & \ding{54} & \\ \hline
gtp.ext\_hdr.pdu\_ses\_con.pdu\_type & & & & & & & & & \ding{54} & \ding{54} \\ \hline
gtp.teid & & & & & & & & & \ding{54} & \ding{54} \\ \hline
http2.amfInstanceId & \ding{54} & & \ding{54} & & & & & & & \\ \hline
http2.ausfInstanceId & \ding{54} & & \ding{54} & & & & & & & \\ \hline
http2.cause & \ding{54} & & \ding{54} & & & & & & & \\ \hline
http2.imsi & \ding{54} & & \ding{54} & & & & & & & \\ \hline
http2.ipv4Address & \ding{54} & & \ding{54} & & & & & & & \\ \hline
http2.jwt.scope & \ding{54} & \ding{54} & \ding{54} & & & & & & & \\ \hline
http2.jwt.sub & \ding{54} & \ding{54} & \ding{54} & & & & & & & \\ \hline
http2.method & \ding{54} & \ding{54} & \ding{54} & & & & & & & \\ \hline
http2.nf-type & \ding{54} & \ding{54} & \ding{54} & & & & & & & \\ \hline
http2.nfInstanceId & \ding{54} & \ding{54} & \ding{54} & & & & & & & \\ \hline
http2.nfType & \ding{54} & \ding{54} & \ding{54} & & & & & & & \\ \hline
http2.path & \ding{54} & \ding{54} & \ding{54} & & & & & & & \\ \hline
http2.request.supi & \ding{54} & & \ding{54} & & & & & & & \\ \hline
http2.requester-nf-type & \ding{54} & \ding{54} & \ding{54} & & & & & & & \\ \hline
http2.service-names & \ding{54} & \ding{54} & \ding{54} & & & & & & & \\ \hline
http2.servingNfId & \ding{54} & \ding{54} & \ding{54} & & & & & & & \\ \hline
http2.subscriberIdentifier & \ding{54} & & \ding{54} & & & & & & & \\ \hline
http2.supis & \ding{54} & & \ding{54} & & & & & & & \\ \hline
http2.supi & \ding{54} & & \ding{54} & & & & & & & \\ \hline
http2.target-nf-instance-id & \ding{54} & \ding{54} & \ding{54} & & & & & & & \\ \hline
http2.target-nf-type & \ding{54} & \ding{54} & \ding{54} & & & & & & & \\ \hline
http2.ueId & \ding{54} & & \ding{54} & & & & & & & \\ \hline
pfcp.apply\_action.drop & & & & & & & \ding{54} & & & \\ \hline
pfcp.apply\_action.forw & & & & & & & \ding{54} & \ding{54} & & \\ \hline
pfcp.cause & & & & \ding{54} & \ding{54} & \ding{54} & \ding{54} & \ding{54} & & \\ \hline
pfcp.f\_seid.ipv4 & & & & \ding{54} & \ding{54} & \ding{54} & \ding{54} & & & \\ \hline
pfcp.f\_teid.ipv4\_addr & & & & & & & \ding{54} & \ding{54} & & \\ \hline
pfcp.f\_teid.teid & & & & \ding{54} & \ding{54} & \ding{54} & \ding{54} & \ding{54} & & \\ \hline
pfcp.far\_id & & & & & \ding{54} & \ding{54} & \ding{54} & \ding{54} & & \\ \hline
pfcp.msg\_type & & & & \ding{54} & \ding{54} & \ding{54} & \ding{54} & \ding{54} & & \\ \hline
pfcp.outer\_hdr\_creation.ipv4 & & & & \ding{54} & & & & & & \\ \hline
pfcp.outer\_hdr\_creation.teid & & & & \ding{54} & \ding{54} & \ding{54} & \ding{54} & \ding{54} & & \\ \hline
pfcp.pdr\_id & & & & \ding{54} & \ding{54} & \ding{54} & \ding{54} & \ding{54} & & \\ \hline
pfcp.seid & & & & \ding{54} & \ding{54} & \ding{54} & \ding{54} & \ding{54} & & \\ \hline
pfcp.ue\_ip\_addr\_ipv4 & & & & & & & \ding{54} & \ding{54} & & \\ \hline
\end{tabular}
\caption{Mapping between the selected features and the attacks in the dataset.}
\label{tab:feature_attack_mapping}
\end{table*}
